# Supplementary material for: NeuroCard: One Cardinality Estimator for All Tables
Source: arXiv:2006.08109 source file (2020-11-02)
Supplement: Supplementary file 1 [file appendix.tex]

\appendix

\section{Hyperparameters}
\begin{table}[h]\centering \small%
\caption{{Hyperparameters of the \sys models reported in Tables~\ref{table:jobl-error} and \ref{table:joblr-error}.}\label{table:workloads}}
\vspace{-.1in}
\begin{tabular}{@{} l l @{}} \toprule
{\textsc{Hyperparam.}} & {\textsc{Value}} \\ \midrule
  ResMADE & ? blocks, each two ?-unit hiddens \\
  ResMADE dropout prob. & ? \\
  Direct I/O layer & ? \\
  Column factorization bits & ? \\
  Embedding size & ? \\
  Tied input/output embeddings & True \\
  Learning rate schedule & ? \\
  Batch size & 2048 \\
  Number of tuples trained & ? \\
  Wildcard skipping & True \\
\bottomrule
\end{tabular}
\end{table}
